# Supplementary material for: Static field-gradient polarizabilities of small atoms and molecules in finite temperature
Source: arXiv:1707.02829 ancillary file (2017-08-11)
Supplement: Supplementary file 1 [file supplementary.pdf]

# Supplementary material

## S1. PIMC DATA OF TEMPERATURE-DEPENDENT TOTAL ENERGIES AND POLARIZABILITIES

TABLE S1. Total energies $E$, dipole–dipole–quadrupole polarizabilities $B$ and quadrupole–quadrupole polarizabilities $C$ of $H_2^+$, $H_2$, $H_3^+$ and $HeH^+$ calculated at variable temperatures and time-steps. 2SEM confidence limits are presented in the parenthesis, and $\tau = 0$ values are obtained by linear extrapolation.

| | | $\tau$ | 50 K | 100 K | 200 K | 400 K | 800 K | 1600 K |
|---|---|---|---|---|---|---|---|---|
| $E$ | $H_2^+$ | 0 | -0.5976(6) | -0.5973(4) | -0.5965(2) | -0.5957(2) | -0.5945(2) | -0.5900(2) |
| | | 0.025 | -0.5972(6) | -0.5969(5) | -0.5965(2) | -0.5958(2) | -0.5945(2) | -0.5900(2) |
| | | 0.05 | -0.5968(5) | -0.5966(4) | -0.59648(14) | -0.59588(13) | -0.5944(2) | -0.58994(13) |
| | $H_2$ | 0 | -1.1620(8) | -1.1636(7) | -1.1631(2) | -1.1624(2) | -1.1613(2) | -1.1584(2) |
| | | 0.025 | -1.1631(9) | -1.1637(7) | -1.1634(2) | -1.1627(2) | -1.1615(2) | -1.1585(3) |
| | | 0.05 | -1.1641(8) | -1.1638(7) | -1.1636(2) | -1.16311(13) | -1.16172(13) | -1.15864(14) |
| | $H_3^+$ | 0 | -1.329(3) | -1.319(4) | -1.3235(6) | -1.3212(4) | -1.3194(5) | -1.3108(4) |
| | | 0.025 | -1.326(2) | -1.322(2) | -1.3230(6) | -1.3214(5) | -1.3195(5) | -1.3114(5) |
| | | 0.05 | -1.324(3) | -1.326(5) | -1.3225(5) | -1.3216(3) | -1.3196(4) | -1.3120(3) |
| | $HeH^+$ | 0 | -2.957(6) | -2.965(3) | -2.9713(10) | -2.9691(11) | -2.9681(9) | -2.9629(9) |
| | | 0.0125 | -2.963(8) | -2.968(3) | -2.9713(10) | -2.9699(13) | -2.9687(10) | -2.9640(11) |
| | | 0.025 | -2.970(4) | -2.971(3) | -2.9713(10) | -2.9708(7) | -2.9692(8) | -2.9651(8) |
| $B$ | $H_2^+$ | 0 | 2617(264) | 1839(157) | 1150(211) | 633(93) | 346(28) | 215(9) |
| | | 0.025 | 2531(286) | 1841(168) | 1142(186) | 636(106) | 347(31) | 216(11) |
| | | 0.05 | 2446(240) | 1842(146) | 1134(234) | 640(77) | 349(24) | 216(7) |
| | $H_2$ | 0 | 150(112) | 123(67) | 55(48) | 6(31) | -34(12) | -60(4) |
| | | 0.025 | 139(116) | 117(71) | 56(55) | 6(33) | -33(14) | -59(4) |
| | | 0.05 | 129(107) | 112(63) | 57(39) | 6(28) | -33(10) | -57(3) |
| | $H_3^+$ | 0 | 775(232) | 549(120) | 398(174) | 223(51) | 113(24) | 71(7) |
| | | 0.025 | 757(280) | 564(131) | 381(198) | 219(60) | 115(29) | 69(8) |
| | | 0.05 | 740(171) | 579(93) | 365(147) | 214(40) | 117(18) | 66(6) |
| | $HeH^+$ | 0 | $1.92(15)\times10^6$ | $7.12(69)\times10^5$ | $2.13(47)\times10^5$ | $5.90(46)\times10^4$ | $1.61(15)\times10^4$ | 4870(260) |
| | | 0.0125 | $1.87(18)\times10^6$ | $6.96(82)\times10^5$ | $2.05(54)\times10^5$ | $5.84(75)\times10^4$ | $1.60(14)\times10^4$ | 4890(250) |
| | | 0.025 | $1.81(12)\times10^6$ | $6.80(53)\times10^5$ | $1.97(39)\times10^5$ | $5.78(49)\times10^4$ | $1.60(15)\times10^4$ | 4900(270) |
| $C$ | $H_2^+$ | 0 | 520(15) | 381(8) | 243(10) | 136(5) | 74(2) | 44.1(4) |
| | | 0.025 | 516(17) | 382(8) | 239(11) | 135(5) | 74(2) | 44.2(5) |
| | | 0.05 | 513(12) | 383(8) | 235(10) | 134(4) | 74(2) | 44.4(3) |
| | $H_2$ | 0 | 30(2) | 28.9(7) | 21.6(5) | 15.8(3) | 11.50(12) | 9.02(5) |
| | | 0.025 | 30(2) | 28.0(7) | 21.9(6) | 15.8(4) | 11.47(14) | 8.99(6) |
| | | 0.05 | 30(2) | 27.1(6) | 22.2(5) | 15.9(3) | 11.44(10) | 8.96(4) |
| | $H_3^+$ | 0 | 160(9) | 127(4) | 88(6) | 54(2) | 30.3(8) | 19.8(2) |
| | | 0.025 | 162(12) | 128(5) | 86(7) | 53(2) | 30(1) | 19.7(3) |
| | | 0.05 | 165(5) | 128(3) | 84(5) | 52(2) | 30.4(6) | 19.6(2) |
| | $HeH^+$ | 0 | 360(17) | 271(17) | 169(17) | 93(5) | 51(2) | 29.0(7) |
| | | 0.0125 | 345(21) | 265(21) | 162(20) | 92(6) | 51(2) | 29.1(7) |
| | | 0.025 | 330(13) | 260(11) | 155(13) | 91(4) | 50(2) | 29.2(8) |

TABLE S2. Fitting parameters and RMSE obtained from the polarizability data presented in Table S1. The form of the fitting function is $f(T) = \left(\frac{a_1 \cdot \mathrm{erf}(a_2 T)}{T}\right)^x + a_3$, where $T$ is the temperature. Two cases for the exponent $x$ are presented: $x$ is either an optimized real number or an integer, *i.e.*, 1 or 2. Inverse squared SEM error estimate has been used in weighting the fitting data and evaluating RMSE.

| | | $x$ | $a_1 \times 10^{-4}$ | $a_2 \times 10^3$ | $a_3$ | RMSE |
|---|---|---|---|---|---|---|
| $B$ | $H_2^+$ | 1 | 20.183 | 12.032 | 89.849 | 0.480 |
| | | 0.88 | 52.505 | 14.876 | 51.238 | 0.333 |
| | $H_2$ | 1 | 3.5532 | 5.4424 | -81.943 | 0.316 |
| | | 0.64 | 60.304 | 8.9310 | -104.44 | 0.116 |
| | $H_3^+$ | 1 | 7.4246 | 8.2232 | 24.465 | 0.365 |
| | | 0.74 | 55.499 | 14.823 | -5.1475 | 0.349 |
| | $HeH^+$ | 2 | 9.1771 | 16.183 | 1628.2 | 1.08 |
| | | 1.84 | 15.366 | 20.177 | 419.88 | 0.224 |
| $C$ | $H_2^+$ | 1 | 4.5974 | 9.8493 | 15.508 | 2.15 |
| | | 0.83 | 13.751 | 13.620 | 3.7497 | 1.29 |
| | $H_2$ | 1 | 0.35446 | 5.9347 | 6.8368 | 2.15 |
| | | 0.75 | 0.87566 | 7.9949 | 5.4521 | 1.12 |
| | $H_3^+$ | 1 | 1.7232 | 7.4011 | 8.9852 | 1.20 |
| | | 0.90 | 2.7370 | 8.4910 | 6.8600 | 1.14 |
| | $HeH^+$ | 1 | 3.3709 | 9.7293 | 8.0405 | 0.796 |
| | | 0.84 | 9.3680 | 12.917 | -0.37037 | 0.298 |
